# Supplementary material for: Direct measurement of the biphoton Wigner function through two-photon interference
Source: arXiv:1304.7092 source file (2013-09-26)
Supplement: Supplementary file 1 [file Douce_SM2.pdf]

# Supplemental Material

PACS numbers: 42.50.-p, 03.65.Ud

## I. MIXED STATES

### A. Entanglement witness

It is straightforward to show that the entanglement witness given by Eq. (4) of the main text is an entanglement witness also for non-pure states $\rho$. Indeed, writing a separable state's density matrix $\rho$ as a convex sum of pure states:

$$\rho = \sum_i \lambda_i |\psi_{1i}\rangle\langle\psi_{1i}| \otimes |\psi_{2i}\rangle\langle\psi_{2i}|, \tag{1}$$

we have $I_\rho(\mu,\delta) = \sum_i \lambda_i I_i(\mu,\delta) \leq 1/2$.

### B. Wigner function

Given a bipartite mixed state $\rho = \sum_i \lambda_i |\psi_{12i}\rangle\langle\psi_{12i}|$, we have

$$I_\rho(\mu,\delta) = \frac{1}{2} - \frac{\pi}{2}\sum_i \lambda_i W_i(\mu,\delta) = \frac{1}{2} - \frac{\pi}{2} W_\rho(\mu,\delta), \tag{2}$$

where $W_\rho(\mu,\delta) = \sum_i \lambda_i W_i(\mu,\delta)$ is the Wigner function of the mixed state.

## II. FOUR DIMENSIONAL WIGNER FUNCTION

### A. General case

The most general (pure) two–photon, two–dimensional wave function can be expressed as:

$$|\psi\rangle = \iint F(p_{x,+}, p_{x,-}, p_{y,+}, p_{y,-}) |p_{1,x}, p_{1,y}, p_{2,x}, p_{2,y}\rangle \mathrm{d}p_{1,x}\mathrm{d}p_{1,y}\mathrm{d}p_{2,x}\mathrm{d}p_{2,y}. \tag{3}$$

where $p_{i\pm} = p_{1,i} \pm p_{2,i}$ with $i = x, y$. By repeating the same calculations developed in the main text and in (11), we have that the coincidences probability is:

$$\begin{aligned} I(\mu_x, \delta_x; \mu_y, \delta_y) = \frac{1}{2} - \frac{\pi^2}{2} \iint & F(\mu_x + p_{x,+}, \mu_x + p_{x,-}, \mu_y + p_{y,+}, \mu_y + p_{y,-}) \times \\ F^*(\mu_x - p_{x,+}, \mu_x - p_{x,-}, \mu_y + p_{y,+}, \mu_y - p_{y,-}) & e^{-2ip_{y,-}\delta_y} e^{-2ip_{x,+}\delta_x} \mathrm{d}p_{y,-}\mathrm{d}p_{y,+}\mathrm{d}p_{x,-}\mathrm{d}p_{x,+}. \end{aligned} \tag{4}$$

Thus, in the general case,

$$I(\mu_x, \delta_x; \mu_y, \delta_y) = \frac{1}{2} - \frac{\pi^2}{2} W(\mu_x, \delta_x, \mu_y, \delta_y). \tag{5}$$

The first pair of coordinates in the equation above refer to the part of the Wigner function that depends on the $x, +$ variables and the second pair to the part of the Wigner function associated to the $y, -$ coordinates. Notice that, by using Dove prisms, as suggested in the main text, one can change the significance of these variables: the first pair will be associated to the $x, -$ function and the second one to the $y, +$ one.

### B. Discussion: Interpretation of Eq. (5)

State (7) can be completely non–separable. In this case, we see from (4) that the Wigner function appearing in (5) reads:

$$W_{r\pm,r_\perp\mp}(\mu_r,\delta_r,\mu_{r_\perp},\delta_{r_\perp}) = \int \mathrm{d}p_{r\pm}p_{r_\perp\mp}\langle\mu_r+p_{r\pm},\mu_{r_\perp}+p_{r_\perp\mp}|\varrho_{r\pm,r_\perp\mp}|\mu_r+p_{r\pm},\mu_{r_\perp}+p_{r_\perp\mp}\rangle e^{2i\delta_r p_{r\pm}}e^{2i\delta_{r_\perp}p_{r_\perp\mp}}, \quad (6)$$

where $\varrho_{r\pm,r_\perp\mp}$ is the reduced density matrix after the trace over variables $r\mp$ and $r_\perp\pm$, with $r$ and $r_\perp$ being two spacial orthogonal coordinates depending on the chosen reflection plane, that can be modified by using a Dove prism.

#### 1. Separable cases

State (7) can be (partially) separable in several ways. We first discuss the case where sum and difference coordinates can be separated but spatial coordinates canont (as in (1) of the main text). The two photon two dimensional wave function is given by:

$$|\psi\rangle = \iint F_+(p_{1,x}+p_{2,x};p_{1,y}+p_{2,y})F_-(p_{1,x}-p_{2,x};p_{1,y}-p_{2,y})|p_{1,x},p_{1,y},p_{2,x},p_{2,y}\rangle \mathrm{d}p_{1,x}\mathrm{d}p_{1,y}\mathrm{d}p_{2,x}\mathrm{d}p_{2,y}, \quad (7)$$

In this case, in Eq. (5), we have that

$$W_{r\pm,r_\perp\mp}(\mu_r,\delta_r,\mu_{r_\perp},\delta_{r_\perp}) = W_{r\pm}(\mu_r,\delta_r)W_{r_\perp\mp}(\mu_{r_\perp},\delta_{r_\perp}) \quad (8)$$

with

$$W_{r\pm}(\mu_r,\delta_r) = \int p_{r_\perp\pm}\langle\mu_r+p_{r\pm}|\varrho_{r\pm}|\mu_r+p_{r\pm}\rangle e^{2i\delta_r p_{r\pm}}, \quad (9)$$

and analogously for the $r_\perp\mp$ coordinate. The density matrix $\varrho_{r\pm}$ ($\varrho_{r_\perp\mp}$) is the trace over the $r_\perp\pm$ ($r\mp$) coordinate. We see that in the case discussed in the main text, we obtained the same expression as (**??**). However, when the state is separable in the spatial coordinates as well, we obtain pure states in (9) instead of mixed ones. In this case, the quantum state can be written as

$$|\psi\rangle = \iint F_{x+}(p_{x+})F_{y+}(p_{y+})F_{x-}(p_{x-})F_{y-}(p_{y-})|p_{1,x},p_{1,y},p_{2,x},p_{2,y}\rangle \mathrm{d}p_{1,x}\mathrm{d}p_{1,y}\mathrm{d}p_{2,x}\mathrm{d}p_{2,y}, \quad (10)$$

Finally, let's discuss the case where states are separable in the spatial coordinate but not in the $+$ and $-$ coordinates, i.e., they can be written in the form:

$$|\psi\rangle = \iint F_x(p_{1,x}+p_{2,x};p_{1,x}-p_{2,x})F_y(p_{1,y}+p_{2,y};p_{1,y}-p_{2,y})|p_{1,x},p_{1,y},p_{2,x},p_{2,y}\rangle \mathrm{d}p_{1,x}\mathrm{d}p_{1,y}\mathrm{d}p_{2,x}\mathrm{d}p_{2,y}, \quad (11)$$

A particular case of this state is the one dimensional distribution, as for example, the frequency states considered in the example discussed in the main text. In this case, Eq. (8) still holds. However, its interpretation is different, since the density matrices $\varrho_{r\pm}$ ($\varrho_{r_\perp\mp}$) are the trace over the $r\mp$ ($r_\perp\pm$) coordinates.

In conclusion, we the modification proposed in the HOM experiment leads to the Wigner function of biphoton state in different coordinates. These coordinates depend on the properties and correlations existing between $+$ and $-$ coordinates of the biphoton, as well as its spatial coordinates.

## III. SYMMETRY OF THE WAVE FUNCTION AND THE WIGNER FUNCTION

It is known that the HOM coincidence detection probability is related to the symmetry properties of the two-photon state. We now connect this to the, also well-known, fact that the Wigner function is related to the symmetry of the *single* particle state. By setting $\delta=\mu=0$, we are measuring the Wigner function at the origin, which is nothing but the average of the parity operator. By writing $F_{x+}(p_+) = (F_{x+,s}(p_+)+F_{x+,a}(p_+))/2$, where $F_{x+,s}(p_+) = (F_{x+}(p_+)+F_{x+}(-p_+))/2$ and $F_{x+,a}(p_+) = (F_{x+}(p_+)-F_{x+}(-p_+))/2$ are the symmetric and anti-symmetric, respectively, parts of $F_{x+,}(p_+)$, we can easily check that $W_{x+}(0,0) = \int |F_{x+,s}(p_+)|^2\mathrm{d}p_+ - \int |F_{x+,a}(p_+)|^2\mathrm{d}p_+$. The same result an be generalized to other coordinates and the 2D case.

## IV. *A POSTERIORI* INTERPRETATION OF OTHER EXPERIMENTS

With the insight provided by our results, we note that Ref. [1] reported the measurement of $I(0,0,0,0)$, and thus the Wigner function at axis $W(0,0,0,0)$ for different pump beams. It is interesting to notice that only when the pump beam was non-gaussian in the $x$ coordinate (and had a negative Wigner function) was it possible to observe $I(0,0,0,0) > 1/2$.

Ref. [2] also reported negative values of the biphoton Wigner function using frequency entangled states. To obtain non gaussian entangled states in this case, it was necessary to create "Schrödinger cat" like states by pumping with a gaussian pump a medium where two distinct phase matching conditions apply. In this case, photons were time delayed with respect to one another. This causes not only a change of visibility in the HOM dip (since when photons are time delayed, they don't arrive at the beam splitter at the same time) but also displaces the point where the Wigner function is calculated.

We notice that our result compares to Ref. [3], in a completely different context. In [3] it was shown that experiment [4] was, in fact, a measure of the Wigner function of the Schödinger cat at the origin of phase space. Analogously, the spatial HOM experiments [1] are also measurements of the biphoton Wigner function at the origin of phase space, and in the frequency version of the HOM experiment [2], the Wigner function in axis $\delta_t$ is measured.

## V. EXTENSION TO MULTI-PHOTON STATES

We now show that our results can be extended to multi-photon states depending on the symmetry properties of the wave functions. We start by a simple example, of four photon states. Denoting $p_i$ the momentum of the $i$-th photon ($i = 1,..,4$) we assume that the wave function can be separated into a product involving four different functions of four independent variables, $p_\alpha$, with $\alpha = A,...,D$ which are linear combinations of $p_i$'s, $i = 1,..,4$. The quantum state, which is the analogous of Eq. (1) of the main text, is thus given by

$$|\psi\rangle = \iiiint F_A(p_A)F_B(p_B)F_C(p_C)F_D(p_D)|p_1,p_2,p_3,p_4\rangle \mathrm{d}p_1\mathrm{d}p_2\mathrm{d}p_3\mathrm{d}p_4. \tag{12}$$

In order to be able to access the Wigner function of one, or several, functions $F_\alpha$, we need that after one, or a combination of several HOM-type experiments, variables $p_\alpha$ either change sign or not, meaning that the transformations performed shall not transform one $p_\alpha$ into a linear combination of other variables $p_{\alpha'}$. In other terms, the HOM experiment measuring the Wigner function can be reformulated as an eigenstate problem, where $p_\alpha$ variables define vectors that are the eigenstates with eigenvalue $\pm 1$. Solving this type of problem and measuring the complete Wigner function is a task that is state dependent, as in the two-photon case detailed in the main text. We will develop in detail a relatively simple case of a multi-photon state that can be completely characterized by our method. Let's consider the $p_\alpha$ variables as follows:

$$p_A = (p_1 + p_2 + p_3 + p_4)/4 \tag{13}$$
$$p_B = (p_1 - p_2 - p_3 + p_4)/4 \tag{14}$$
$$p_C = (p_1 + p_2 - p_3 - p_4)/4 \tag{15}$$
$$p_D = (p_1 - p_2 + p_3 - p_4)/4 \tag{16}$$

We can start by sending each one of the $i$ photons in one entry of the set-up shown in Fig. 1. For the sake of simplicity we will restrict ourselves to the description of the $x$ variables only. Following the same reasoning as in the two–photon case, we have that interfering paths 1 and 2 in a HOM set–up can interchange variables $p_1$ and $p_2$ and change their signs, because of reflection in the BS. Independently, variables 3 and 4 are also interchanged and change their sign in the HOM configuration involving these two arms only. The same calculations as the one realized in the two photon case can be carried on. If position displacements $\delta_i$ are realized in arms $i = 1,3$ and momentum displacements $\mu_i$ are realized in arms $i = 2,4$, as in Figure 1, we have that the probability of detecting coincidences in the four detectors $D_\alpha$ is proportional to

$$\begin{aligned}
&\iiiint F_A(p_A+\mu_A)F_A^*(-p_A+\mu_A)F_C(p_C+\mu_C)F_C^*(-p_C+\mu_C)\times \\
&|F_B(p_B+\mu)|^2|F_D(p_D+\mu)|^2 e^{-i(p_A\delta_A+p_C\delta_C)}\mathrm{d}p_A\mathrm{d}p_B\mathrm{d}p_C\mathrm{d}p_D + \\
&\iiiint F_A(p_A)F_A^*(p_C+2\mu_4)F_C(p_C)F_C^*(p_A+2\mu_2)|F(p_B)|^2|F(p_D)|^2 e^{i(p_A-p_c)\delta_3/2}\mathrm{d}p_A\mathrm{d}p_B\mathrm{d}p_C\mathrm{d}p_D + \\
&\iiiint F_A(p_A)F_A^*(-p_C-2\mu_4)F_C(p_C)F_C^*(-p_A-2\mu_2)|F(p_B)|^2|F(p_D)|^2 e^{i(p_A+p_c)\delta_1/2}\mathrm{d}p_A\mathrm{d}p_B\mathrm{d}p_C\mathrm{d}p_D
\end{aligned} \tag{17}$$

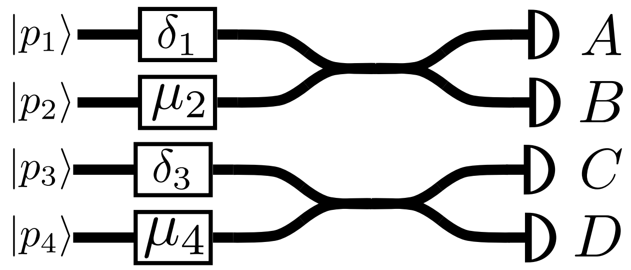


FIG. 1: HOM type experiment with simultaneous and independent interference between paths 1 and 2 and 3 and 4, respectively

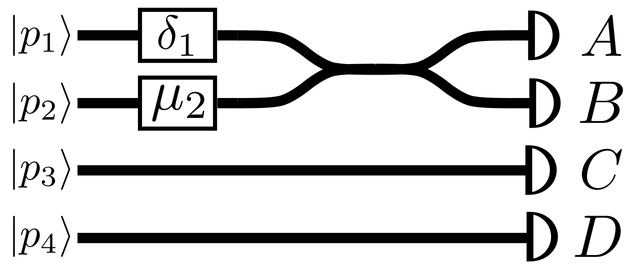


FIG. 2: HOM type experiment interfering paths 1 and 2. A complementary experiment to the one realized in Fig. 1 leading to the determination of extra interference terms of the coincidence probability obtained in the experiment described by Fig. 1

where $\delta_A = (\delta_1 + \delta_3)/2$, $\delta_C = (\delta 1 - \delta_3)/2$, $\mu_A = \mu_2 + \mu_4$ and $\mu_C = \mu_2 - \mu_4$. Supposing that functions $F_\alpha$ are normalized to 1, Eq. (17) becomes proportional to:

$$\begin{aligned} &\pi^2 W_A(\mu_A, \delta_A/2) W_C(\mu_C, \delta_C/2) - \\ &\iint F_A(p_A) F_A^*(p_C + 2\mu_4) F_C(p_C) F_C^*(p_A + 2\mu_2) e^{i(p_A - p_c)\delta_3/2} \mathrm{d}p_A \mathrm{d}p_C - \\ &\iint F_A(p_A) F_A^*(-p_C - 2\mu_4) F_C(p_C) F_C^*(-p_A - 2\mu_2) e^{i(p_A + p_c)\delta_1/2} \mathrm{d}p_A \mathrm{d}p_C \end{aligned} \tag{18}$$

It is clear that only the first term leads to the Wigner function associated to functions $F_A$ and $F_C$. It is possible to access this information and isolate this term only by realizing other independent HOM experiments where either arms 1 and 2 or arms 3 and 4 interfere, as depicted in Figs. 2 and 3. These two experiments corresponds to terms 2 and 3 of Eq. (18) and by subtracting them from the coincidence signal obtained when realizing the experiment in Fig. 1, once can access the product of the Wigner function associated to $F_A$ and $F_C$.

Obtaining the Wigner function associated to $F_B$ and $F_D$ can be done in a similar way. In order to do so, one can, for instance, use a Dove prism, as in the two–photon case, and map the $x$ distribution into the $y$ axis, that doesn't change sign upon reflexion. Applying the procedure described above, *i.e.*, making two simultaneous HOM involving arms $1,2$ and $3,4$, then subtracting from the obtained coincidence probability, the coincidence probability of two other HOM experiments involving the interference of arms $1,2$ or $3,4$, leads to the product of the Wigner function associated to functions $F_B$ and $F_D$. This information, together with the previously obtained one on $W_A W_C$, allows for the complete characterization of state (12). We recall that we chose a relatively simple example to detail in this section, in order to point out that the proposed method to directly measure the Wigner function also applies to multi-photon states. Other examples of multi-photon states can also be completely characterized if they're described by wave functions which are separable in variables that are eigenstates with negative eigenvalues of the HOM transformation in either $x$ or $y$ directions. In other cases, the presented method still works, but returns, analogously to what has been shown in Section I of this Supplemental Material, the Wigner function of a non-pure state.

## VI. POSITION AND MOMENTUM TRANSLATIONS

Transverse position and momentum translations can be performed in a number of ways. These translations correspond to shifts in the near-field (position $x$) and far-field (momentum $p$) spatial variables of an optical field. In Ref.

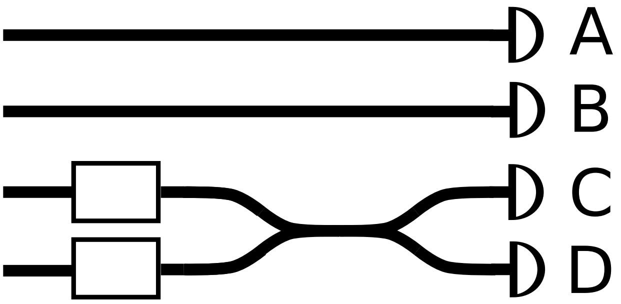


FIG. 3: HOM type experiment interfering paths 3 and 4. A complementary experiment to the one realized in Fig. 1 leading to the determination of extra interference terms of the coincidence probability obtained in the experiment described by Fig. 1

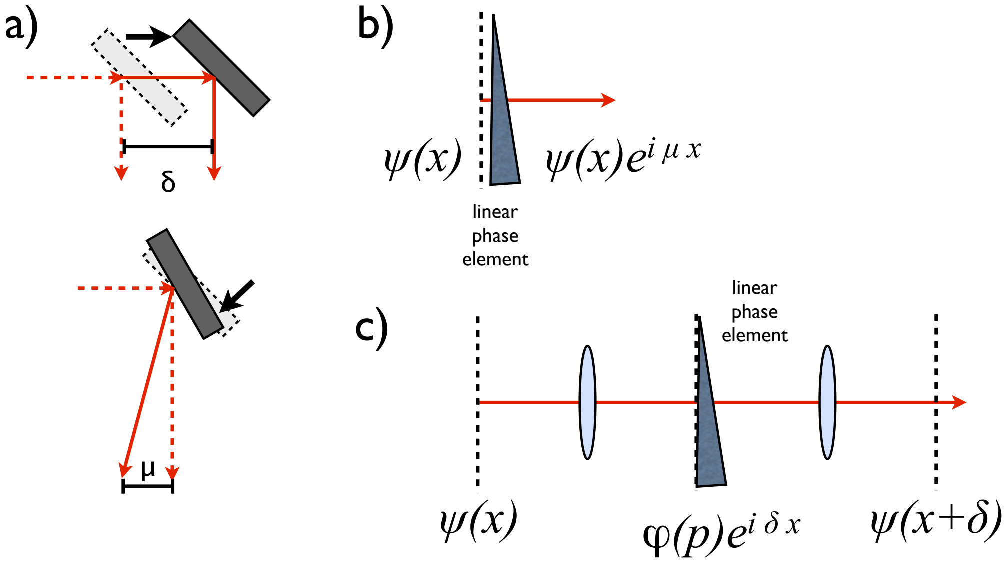


FIG. 4: Methods to implement position and momentum translations. In a), a mirror is shifted and/or tilted to cause a position shift $\delta$ and/or mometum shift $\mu$. Using a linear phase element, a momentum shift or position shift can be implemented as in b) or c), respectively. In c), the phase element is placed at the focal plane of two confocal lenses.

[5] this was performed by shifting the position and/or the angle of a steering mirror, as illustrated in Fig. 4 a). In this way, the Wigner function was reconstructed as a function of the position shift $\delta$ and momentum shift $\mu$.

Another method to perform a momentum shift is shown in Fig. 4 b). It involves imprinting a linear position-dependent phase $\exp ix\mu$ on the field, so that $\psi(x) \longrightarrow \psi(x)\exp(ix\mu)$. The linear phase can be applied using a spatial light modulator (SLM), or a material where the optical length of the medium varies linearly with $x$, as described in Ref. [6]. The Fourier transform of this field is $\varphi\psi(p+\mu)$, which displays the momentum shift. Imprinting this phase at a plane located between two lenses in a confocal arrangement, as drawn in Fig. 4 c) is equivalent to a linear phase in momentum space, corresponding to a position shift: $\psi(x) \longrightarrow \psi(x+\delta)$.

[1] S. P. Walborn, A. N. de Oliveira, S. Padua, C. H. Monken, Phys. Rev. Lett **90**, 143601 (2003).
[2] A. Eckstein and C. Silberhorn, Opt. Lett. **33**, 1825 (2008).
[3] L. G. Lutterbach and L. Davidovich, Phys. Rev. Lett. **78**, 2547 (1997).
[4] M. Brune, *et al.*, Phys. Rev. Lett. **77**, 4887 (1996); L. Davidovich *et al.*, Phys. Rev. A **53**, 1295 (1996).
[5] E. Mukamel, K. Banaszek, I. A. Walmsley and C. Dorrer, Opt. Lett. **28**, 1317 (2003).
[6] D. Tasca, *et al.*, Phys. Rev. A **83**, 052325 (2011).
